# Supplementary material for: Dense Voxel Fusion for 3D Object Detection
Source: arXiv:2203.00871 source file (2022-10-27)
Supplement: Supplementary file 1 [file appendix.tex]

\setcounter{table}{7}
\setcounter{figure}{4}

\begin{table*}[t]
\centering
\begin{tabular}{c|ccc|ccc|ccc}
\toprule
                              & \multicolumn{3}{c|}{Inference 2D Detector} & \multicolumn{3}{c|}{3D AP}                                                                    & \multicolumn{3}{c}{BEV AP} \\
\multirow{-2}{*}{Method}      & Model      & Pretrained     & Fine-tune    & Easy                          & Mod.                          & Hard                          & Easy    & Mod.    & Hard   \\ \hline
PV-RCNN~\cite{PVRCNN}                       & N/A        & N/A            & N/A          & \cellcolor[HTML]{FFFFFF}91.88 & \cellcolor[HTML]{FFFFFF}84.83 & \cellcolor[HTML]{FFFFFF}82.55 & 93.73   & 90.65   & 88.55  \\ \hline
                              & C-RCNN     & COCO           & Yes          & \cellcolor[HTML]{FFFFFF}92.81 & \cellcolor[HTML]{FFFFFF}85.53 & \cellcolor[HTML]{FFFFFF}83.01 & 95.85   & 91.22   & 88.94  \\
                              & C-RCNN     & COCO           & No           & \cellcolor[HTML]{FFFFFF}92.55 & \cellcolor[HTML]{FFFFFF}85.37 & \cellcolor[HTML]{FFFFFF}82.92 & 95.32   & 91.26   & 88.93  \\ 
                              & M-RCNN     & Cityscapes     & Yes          & \cellcolor[HTML]{FFFFFF}92.90 & \cellcolor[HTML]{FFFFFF}85.39 & \cellcolor[HTML]{FFFFFF}83.00 & 95.91   & 91.27   & 88.97  \\
\multirow{-4}{*}{DVF+PV-RCNN} & M-RCNN     & Cityscapes     & No           & \cellcolor[HTML]{FFFFFF}92.95 & \cellcolor[HTML]{FFFFFF}85.47 & \cellcolor[HTML]{FFFFFF}82.94 & 96.02   & 91.32   & 88.95  \\ \bottomrule
\end{tabular}
  \caption{3D and BEV $AP |_{R_{40}}$ results on KITTI~\cite{Kitti} \textit{val} set of a single \method+PV-RCNN trained model using multiple 2D detectors at inference time. Two models are considered; Cascade-RCNN~\cite{crcnn} \textbf{C-RCNN} and Mask-RCNN~\cite{mrcnn} \textbf{M-RCNN}. \textbf{C-RCNN} models are pretrained on COCO dataset~\cite{coco} and \textbf{M-RCNN} are pretrained on Cityscapes dataset~\cite{cityscapes}. Finally, the same models are fine-tuned on images in KITTI~\cite{Kitti} \textit{train} set.}
  \label{tab:no_training}
\end{table*}

\begin{table}
\centering
\resizebox{\columnwidth}{!}{
\begin{tabular}{c|ccc|ccc}
\toprule
\multirow{3}{*}{Method} & \multicolumn{3}{c|}{C-RCNN}                      & \multicolumn{3}{c}{GT}                           \\
                        & \multicolumn{3}{c|}{Car - 3D AP}                 & \multicolumn{3}{c}{Car - 3D AP}                  \\
                        & 0-20m          & 20-40m         & 40-Inf         & 0-20m          & 20-40m         & 40-Inf         \\ \hline
Painted PV-RCNN         & 88.13          & 81.39          & 30.38          & 93.15          & 84.23          & 35.70          \\
DVF+PV-RCNN             & \textbf{90.62} & \textbf{81.48} & \textbf{32.03} & \textbf{93.60} & \textbf{85.29} & \textbf{40.75} \\
\rowcolor{LightCyan}\textit{Improvement}             & +2.49          & +0.09          & +1.65          & +0.45          & +1.06          & +5.05          \\ \bottomrule
\end{tabular}}
  \caption{Range-based evaluation of Pointpainting~\cite{pointpainting} and \method applied to PV-RCNN~\cite{PVRCNN}. The same training strategy is used for both fusion methods. Inference on the KITTI \textit{val} set is performed using both using Cascade-RCNN~\cite{crcnn} 2D predictions \textbf{C-RCNN} and ground truth 2D bounding boxes \textbf{GT}. Improvements in 3D$AP|_{R_{40}}$ are shown relative to painted models.}
  \label{tab:range_based_dvf}
\end{table}

\begin{figure*}[h]
  \centering
  \includegraphics[width=1.0\linewidth]{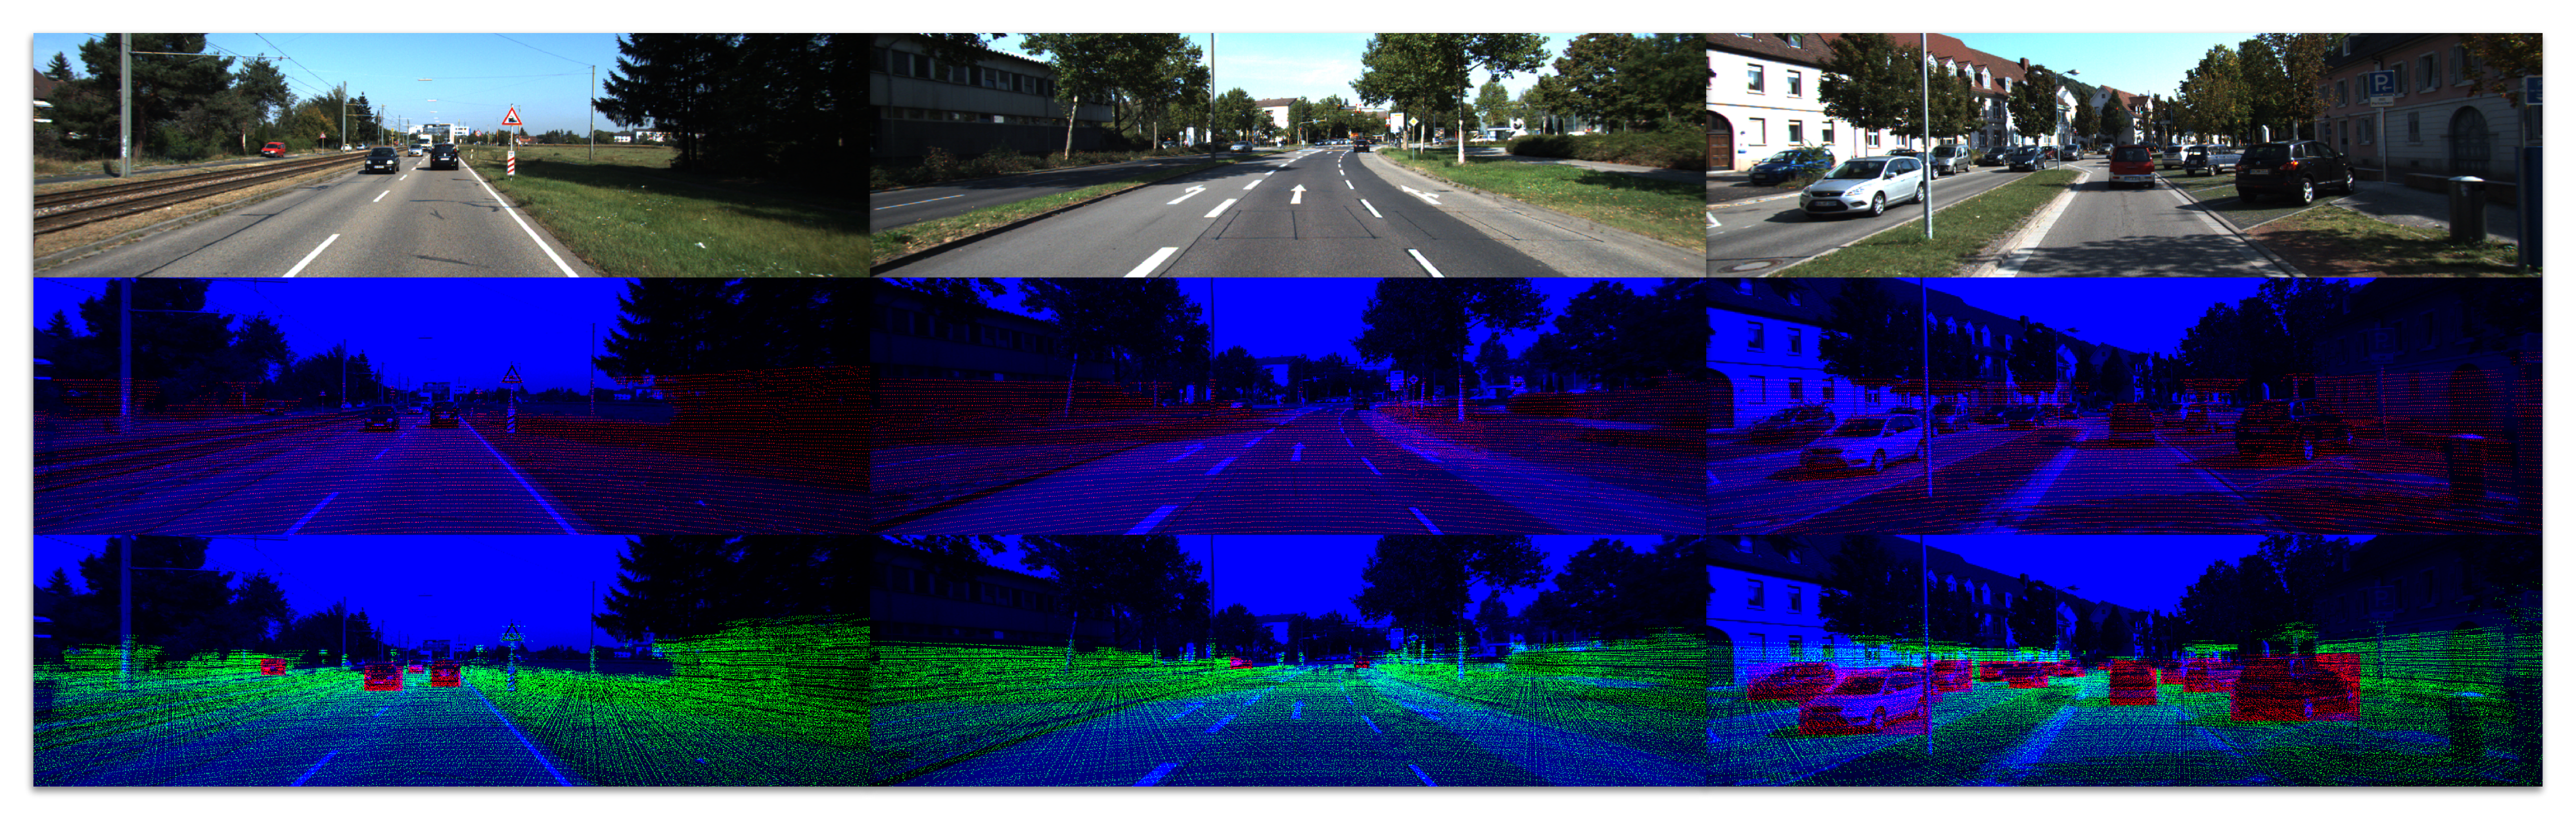}
   \caption{First row shows input images from KITTI~\cite{Kitti} dataset, second row shows \textcolor{red}{\textbf{red}} points represent LiDAR returns projected onto the image plane, and third row shows multi-scale dense voxel centers projected onto the image plane, where \textcolor{DarkGreen}{\textbf{green}} and \textcolor{red}{\textbf{red}} points are associated with background and foreground voxel features respectively. \method increases the number of correspondences between image and LiDAR features which improves detection at mid-to-long range.}
   \label{fig:dense_fusion_examples}
\end{figure*}

\label{sec:dvf_vis}
This supplementary material contains the following five sections. In Section~\ref{sec:inference_pretrained} we demonstrate that training \method using ground truth projected 3D labels can generalize to multiple 2D detectors, including detectors that are not fine-tuned on KITTI \textit{train} set. In Section~\ref{sec:range_evaluation} we conduct a range-based evaluation of \method and show significant improvements over sparse fusion at far range. In Section~\ref{sec:sim_conf} we discuss the effect of the simulated confidence sampling strategy on the performance of \method models. In Section~\ref{sec:dropout} we discuss the effect of the drop-out percentage on the performance of \method models. In Section~\ref{sec:std} we present the standard deviation of \method models trained on KITTI dataset. In Section~\ref{sec:dvf_vis} we provide more examples for visualizing \method. In Sections~\ref{sec:limit} we discuss limitations of the proposed method and discuss potential solutions. Finally, in Section~\ref{sec:negative} we briefly discuss potential negative impact of our work.
\section{Inference using Pretrained 2D Object Detectors}
\label{sec:inference_pretrained}
% Purpose of this experiments
One of the advantages of training \method models directly with ground truth projected 3D bounding box labels rather than noisy, detector-specific, 2D predictions, is that it enables the generalization to any 2D object detector during inference time. To show this, instead of using CLOCs 2D predictions~\cite{clocs}, we train a single \method+PV-RCNN using ground truth labels and conduct inference using multiple 2D object detectors. Specifically, we use Detectron2~\cite{detectron2} pretrained Cascade-RCNN~\cite{crcnn} and Mask-RCNN~\cite{mrcnn} models with ResNet-50~\cite{deepResidualNetworks} backbone to extract 2D predictions without fine-tuning on KITTI images. In addition, we fine-tune the same models on KITTI \textit{train} set and show 3D and BEV $AP |_{R_{40}}$ on \textit{val} set compared to models that are not fine-tuned on KITTI \textit{train} set. In~\Cref{tab:no_training} we observe that the trained model \method+PV-RCNN gains are consistent compared to the baseline PV-RCNN~\cite{PVRCNN} regardless of the pretrained 2D model.  In addition, due to the small size of KITTI \textit{train} set, fine-tuning does not have a significant advantage over using predictions from pretrained 2D object detectors. 
\section{Range-based Evaluation}
\label{sec:range_evaluation}
\method fuses at the voxel level which augments LiDAR point cloud information with dense details from image data. This is contrary to Pointpainting~\cite{pointpainting} where fusion is at the 3D point level, and is therefore sparse, especially at mid-to-long range. We show that dense fusion is especially useful at mid-to-long range, where more objects are occluded and LiDAR returns are sparse. In~\Cref{tab:range_based_dvf} we conduct a range-based evaluation for the 3D predictions of Pointpainting~\cite{pointpainting} and \method applied to PV-RCNN~\cite{PVRCNN}. We evaluate 3D AP $|_{R_{40}}$ on three range bins $[0.0, 20.0]$m, $[20.0, 40.0]$m and greater than $40$m. Inference is done using 2D predictions from Cascade-RCNN~\cite{crcnn}. In addition, we conduct inference using ground truth 2D bounding boxes for both models to determine an upper bound on the potential gains for Pointpainting and \method. Dense voxel fusion shows significant improvement over Pointpainting~\cite{pointpainting} of +1.65\% and +5.05\% at long range (i.e., greater than $40$m ) using Cascade-RCNN~\cite{crcnn} 2D predictions and ground truth labels respectively. 
\begin{figure}[h!]
  \centering
  \includegraphics[width=1.0\linewidth]{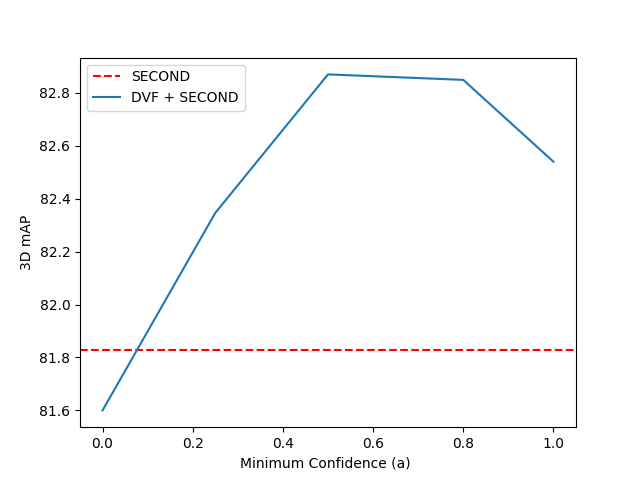}
   \caption{The effect of the minimum confidence on the performance of \method + SECOND~\cite{SECOND}. Here, we also show the performance of the baseline.}
   \label{fig:min_confidence}
\end{figure}
\begin{figure}[h!]
  \centering
  \includegraphics[width=1.0\linewidth]{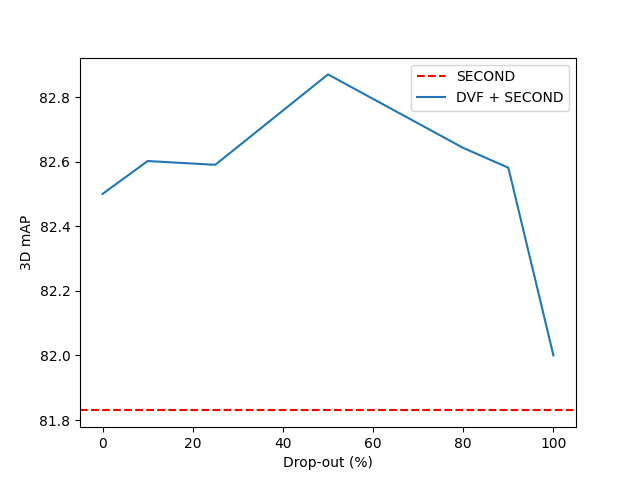}
   \caption{The effect of the drop-out percentage on the performance of \method + SECOND~\cite{SECOND}. Here, we also show the performance of the baseline.}
   \label{fig:gt_dropout}
\end{figure}
\section{Effect of Simulated Confidence}
% Describe experiment
\label{sec:sim_conf}
To study the effect of the simulated confidence of the projected 3D bounding boxes on the performance of \method models, we conduct an experiment using SECOND~\cite{SECOND} where we vary the minimum confidence value $a$ from $0.0$ to $1.0$, while the maximum confidence $b$ is fixed at $1.0$. For each experiment, we drop-out $50\%$ of the ground truth samples added to each scene to simulate missed image detections. Looking at \Cref{fig:min_confidence}, we observe that low confidence values result in poor performance since missed detections are already simulated using the drop-out strategy. In addition, very high $a$ results in simulating an overly confident 2D object detector. The optimal values for SECOND~\cite{SECOND} are around $[0.5, 0.8]$. The minimum simulated confidence is set at $0.8$ for all our experiments. We have also experimented with sampling confidence values proportional to the size of the projected 3D bounding box, but did not achieve better results over the presented uniform sampling strategy. 
\section{Effect of Drop-out Percentage}
\label{sec:dropout}
% Describe experiment
During the training of \method models, a percentage of the objects (i.e., ground truth samples) added to the point cloud, are not projected back to the foreground mask. The goal here is to simulate image missed detections. To study the effect of the drop-out percentage on the performance of \method models, we conduct an experiment using SECOND~\cite{SECOND} where we vary the drop-out percentage of the ground truth samples from $0\%$ to $100\%$. Here, we set the maximum number of added ground truth samples per scene to $5.0$. Similar to the implementation of ground truth sampling in OpenPCDet~\cite{openpcdet2020} library, only samples that do not collide with other samples in the current scene are added. Looking at ~\Cref{fig:gt_dropout} we observe that dropping $100\%$ of the added ground truth samples from the foreground mask results in a model that achieves almost the same performance as the baseline. We reason that the model learns to ignore the image information as it misses many objects that can be easily detected from the LiDAR data. On the other hand, setting the drop-out percentage $0.0\%$ results in a model that relies too much on image information and thus is not robust against image missed detections. Dropping around $50\%$ of the ground truth samples from the foreground mask is a good compromise. We set the drop-out percentage to $50\%$ for all our experiments.  
\section{Standard Deviation of Experiments}
\label{sec:std}
%%%% Standard deviation of main results %%%%%
\Cref{tab:baseline_car_std} shows the standard deviation of \method models. The standard deviation is computed based on running 3 experiments for each model. In addition, we also report the improvement relative to the baseline models. 
\begin{table}[t]
\centering
\resizebox{\columnwidth}{!}{
\begin{tabular}{c|ccc|ccc}
\toprule
                                         & \multicolumn{3}{c|}{Car - 3D AP}                                                                                         & \multicolumn{3}{c}{Car - BEV AP}                 \\
\multirow{-2}{*}{Method}                 & Easy                                   & Mod.                                   & Hard                                   & Easy           & Mod.           & Hard           \\ \hline
\method + SECOND                                   & 0.43                                  & 0.24                                  & 0.19                                  & 0.51           & 0.34          & 0.11          \\
\rowcolor{LightCyan} 
\textit{Improvement}                     &1.74                          &1.01                          &0.71                          &1.83  & 0.83  & 0.30   \\ \hline
\cellcolor[HTML]{FFFFFF}\method + Voxel-RCNN       & \cellcolor[HTML]{FFFFFF}0.12          & \cellcolor[HTML]{FFFFFF}0.09           & \cellcolor[HTML]{FFFFFF}0.10          &0.15          &0.11           &0.12          \\
\rowcolor{LightCyan}
\textit{Improvement}                     & 0.52                          &0.61                          &0.31                          &0.66  &0.63  & 0.54  \\ \hline
\cellcolor[HTML]{FFFFFF}\method + PV-RCNN          & \cellcolor[HTML]{FFFFFF}0.23          & \cellcolor[HTML]{FFFFFF}0.12          & \cellcolor[HTML]{FFFFFF}0.08          &0.04          &0.11          &0.07          \\
\rowcolor{LightCyan} 
\textit{Improvement}                     &1.19                          &1.01                          &0.58                          &2.48  &1.01  & 0.62  \\ \bottomrule
\end{tabular}}
\caption{The standard deviation of 3D and BEV AP $|_{R_{40}}$ on KITTI \textit{val} set for \method models on car class. The improvement relative to the baseline is also presented.}

\label{tab:baseline_car_std}
\end{table}
\section{\method Visualization}
\label{sec:dvf_vis}
\Cref{fig:dense_fusion_examples} shows how \method increases the number of correspondences between LiDAR point cloud and image pixels. Here, the second row shows the sparse point cloud projected onto the image plane. In the last row, we project voxel centers associated with occupied voxels onto 2D predicted foreground mask. Voxel centers with a foreground probability of more than 0.9 are colored in red, while the remaining voxels are considered background and are colored in green.
\section{Limitations}
\label{sec:limit}
\noindent \textbf{Training Strategy.}
Our training strategy consists of training with ground truth 2D bounding boxes while simulating image missed detections throughout the training phase. We have demonstrated that training using this strategy generalizes better than training with erroneous 2D predictions. However, our proposed training strategy does not simulate errors in bounding box dimensions. One possible approach to address this limitation is to train \method models by adding random noise to the center, width and height of ground truth 2D boxes to simulate small shifts in 2D predictions. Moreover, we could also simulate 2D prediction confidence based on occlusion, size and number of LiDAR returns per 3D bounding box. 
\\[0.2\baselineskip]
% 2D bounding boxes are faster than using segmentation but are two large for close enough objects
\noindent \textbf{Object Boundaries.} One of the main advantages of using 2D bounding boxes for fusion compared to segmentation masks is the efficient inference time of 2D object detectors compared to segmentation networks. However, 2D bounding boxes do not capture object boundaries and thus are less accurate than segmentation masks. Hence, background voxels around bounding box boundaries are incorrectly weighted as foreground voxels. One possible approach to address to address this limitation is by modelling 2D bounding box detections as a mixture of Gaussian distributions. The intuition is that our confidence of whether a pixel is foreground or background within a bounding box falls off as we move away from the center of the bounding box. The parameters of each Gaussian distribution corresponding to a 2D prediction can be learned based on the width, height and depth distribution of LiDAR points within the bounding box. 

\section{Potential Negative Impact}
\label{sec:negative}
% surveillance for policing and targetting protestors
Some potential negative impacts of 3D object detectors include using models for ethically questionable surveillance applications like detecting, counting, and tracking of peaceful demonstrators. Therefore, it is critical to enforce the anonymization of the input sensor data. For example, license plates of vehicles and faces of pedestrians and cyclists should be completely anonimized before conducting inference.
